# Supplementary material for: Hybrid Modal Operators for Definite Descriptions
Source: arXiv:2410.10439 source file (2024-10-14)
Supplement: Supplementary file 1 [file appendix.tex]

\newpage

\appendix

\section{Proof details}

\noindent \textbf{\Cref{lem:game}}\quad
\emph{For any $\MLi$-formula $\varphi$ with Boolean \DD{}s, $\varphi$ is satisfiable if and only if  Eloise has a winning strategy in the $\varphi$-game.}\medskip

\begin{proof}
If $\varphi$ is satisfiable, then $\M,w_0 \models \varphi$, for some model $\M=(W,R,V)$ and $w_0 \in W$.
Let $w_1, \dots, w_n \in W$ be all the worlds which satisfy formulas from $\iota(\varphi)$; moreover,  for any $w \in W$, let $H(w)$ be the unique $\varphi$-Hintikka set that contains all  formulas in $\cl(\varphi)$ which are satisfied at $w$ in $\M$.
The winning strategy for Eloise
is to start by playing the set $\Hs = \{ H(w_0), \dots, H(w_n) \}$ and the relation on $\Hs$ which is the projection of $R$ on $\{w_0, \dots, w_n \}$.
Then, if Abelard plays a set $H(w_k) \in \Hs$ and a formula $\Diamond \varphi' \in H(w_k)$,
Eloise replays by playing  $H(w_\ell)$ for  any $w_\ell \in W$ such that $R(w_k,w_\ell)$ and $\M, w_\ell \models \varphi'$.
Such $w_\ell$ is guaranteed to exist and $H(w_\ell)$ satisfies the conditions listed in the game description.
Since the game always terminates, this  strategy is indeed winning for Eloise.

For the opposite implication assume that Eloise has a winning strategy in which she starts by playing $\Hs_0 = \{H_0, \dots, H_n \}$.
% We will consider the hardest case, in which the game can take the maximal number of  turns, namely $\md(\varphi) +1 $ turns of Abelard.
% In this case, 
We define sets $\Hs_1, \dots, \Hs_{\md(\varphi)}$ such that each $\Hs_{k+1}$ contains
all $\varphi$-Hintikka sets not belonging to $\Hs_0$ which Eloise would play (using the winning strategy)
as a response to Abelard playing some set (and a formula) in $\Hs_k$.
We exploit these $\Hs_0, \dots, \Hs_{\md(\varphi)}$ to construct a model $\M=(W,R,V)$  such that 
\begin{align*}
W & = \{ w_k^H \mid k \in \{0, \dots, \md(\varphi) \} \text{ and } H \in \Hs_k \},
\\
R & = \{ (w_k^H, w_{k'}^{H'}) \in W \times W  \mid \psi \in w_{k'}^{H'} \text{ implies } \Diamond \psi \in w_k^H, \text{ for all } \Diamond \psi \in \cl(\varphi) \},
\\
V(p) & = \{w_k^H \in W \mid p \in H \}, \quad \text{ for each } p \in \prop.
\end{align*}
Now, we will show by induction on the structure (treated as the number of symbols used to write the formula) of formulas 
that for any 
$w_k^H \in W$
and any 
$\psi \in \cl(\varphi)$  with $\md(\psi) \leq \md(\varphi) -k $ the following statement holds:

\smallskip

\centerline{$\M, w_k^H \models \psi$ if and only if $\psi \in H$.}

\smallskip

\noindent 
If $\psi \in \prop$, then the statement holds by the definition of $V$.
If $\psi$ is of the form $\neg \psi'$ or $\psi' \lor \psi''$, then the statement holds by the inductive assumption and the fact that $H$ is a $\varphi$-Hintikka set.

Next, we consider $\psi$ of the form $\Diamond \psi'$ and we assume that $\Diamond \psi' \not\in H$.
To show  that $\M, w_k^H \not\models \Diamond \psi'$
we fix an arbitrary $w_{k'}^{H'} \in W$ such that $R(w_k^H,w_{k'}^{H'})$; by the definition of $R$ we have $\psi \notin w_{k'}^{H'}$, and so, by the inductive assumption and the arbitrariness of $w_{k'}^{H'}$ we conclude that 
$\M, w_{k}^{H} \not\models \Diamond \psi'$. 
For the opposite direction assume that
$\Diamond \psi' \in H$.
As $\md (\Diamond \psi') \geq 1$,
we have $k +1 \leq \md(\varphi)$, and so
Abelard could play $H$ and $\Diamond \psi'$ in his $k+1$st turn (recall that Abelard can play at most $\md(\varphi)+1$ turns).
Hence Eloise's winning strategy needs to 
provide $H'$ such that
$\psi' \in H'$ and
for all $\Diamond \chi \in \cl(\varphi)$ if $\chi \in H'$, then $\Diamond \chi \in H$.
Thus, by the definition of $R$, we have $R(w_k^H,w_{k+1}^{H'})$.
Since $\psi \in H'$, by the inductive assumption  we obtain that $\M,w_{k+1}^{H'} \models \psi'$, so $\M, w_k^H \models \Diamond \psi'$.

Finally, consider $\psi$  of the form $@_{\iota \chi} \eta$.
If $\M, w_k^H \models \psi$, then there exists  $w_{k'}^{H'}$ such that $\M, w_{k'}^{H'} \models \chi \land \eta$.
As we consider only Boolean \DD{}s, we have that $\md(\chi)=0$, and so,  by the inductive assumption we obtain that  $\chi \in H'$.
Thus, by the definition of the game, we have $k'=0$.
Therefore $\md(\eta) \leq \md(\varphi) - k'$ and the inductive assumption applies to $\M, w_{k'}^{H'} \models  \eta$, which yields $\eta \in H'$.
The fact that $k'=0$ and $\{ \chi,\eta \} \in H'$ implies, by the conditions imposed in the game on the initial set $\Hs_0$, that $@_{\iota \chi} \eta \in H'$.

If $@_{\iota \chi} \eta \in H$ then, by the definition of the game,
there needs to exist  $w_{k'}^{H'} \in W$ such that $\{ \chi, \eta \} \subseteq H'$ and $k'=0$.
%As $\md(\chi) \leq \md(\varphi)$ and $\md(\eta) \leq \md(\varphi)$, 
Then, by the inductive assumption, we obtain that
$\M,w_{0}^{H'} \models \chi$ and $\M, w_0^{H'} \models \eta$.
To show that $\M, w_k^H \models @_{\iota \chi} \eta$ we need to additionally argue that there is no $w_{k''}^{H''} \in W$ such that $w_{k''}^{H''} \neq w_{k'}^{H'}$  and $\M, w_{k''}^{H''}\models   \chi $. 
Suppose towards a contradiction that there exists such 
$w_{k''}^{H''}$.
Since we consider Boolean \DD{}s only, $\md(\chi)=0$.
Hence,   we get by the inductive assumption that
$\chi \in H''$.
Thus, by the definition of the game, it must be the case that $k''=0$.
This, however, violates the condition that each formula in $\iotaf(\varphi)$ can occur in at most one $H \in \Hs_0$. 
%
% If such $w_{k''}^{H''}$ did exist, then \pw{This is not true that $k''=0-$}$k''=0$, whereas the definition of the first move of Eloise implies that $H'=H''$. This, however means that $w_{k''}^{H''} = w_{k'}^{H'}$, which raises a contradiction.
\qed
\end{proof}

%\subsection*{Proof of \Cref{expt}}

\noindent \textbf{\Cref{expt}}\quad
\emph{Checking satisfiability of \MLi{}-formulas (with arbitrarily complex \DD{}s) is \EXPT{}-complete.}\medskip

\begin{proof}

We will provide the missing details of the inductive proofs mentioned in the main body of the paper.

Let us conduct the induction for the left-to-right implication first.\smallskip

\noindent $\psi=p$ or $\psi=\neg p$\quad Assume that $\M,w\models\psi$. Of course $w$. Since, by the definition of $\tau$, $\tau(\psi)=\psi$ and $V(p)=V'(p)$, we get $\M',w\models\tau(\psi)$.\smallskip

\noindent $\psi=\chi\land\theta$\quad Assume that $\M,w\models\chi\land\theta$. Hence, we have $\M,w\models\chi$ and $\M,w\models\theta$. By the inductive assumption, $\M',w\models\tau(\chi)$ and $\M',w\models\tau(\theta)$ and further, by the definition of $\tau$, $\M',w\models\tau(\chi\land\theta)$. The case where $\psi=\chi\lor\theta$ is proceeded similarly.\smallskip

\noindent $\psi=\Diamond\chi$\quad Assume that $\M,w\models\Diamond\chi$. It means that there exists $v\in W$ such that $(w,v)\in R$ and $\M,v\models\chi$. By the inductive assumption, $\M',v\models\tau(\chi)$, and so, $\M',w\models\Diamond\tau(\chi)$. Hence, by the definition of $\tau$, $\M',v\models\tau(\Diamond\chi)$.\smallskip

\noindent $\psi=\Box\chi$\quad Assume that $\M,w\models\Box\chi$. It means that, for all $v\in W$ such that $(w,v)\in R$, it holds $\M,v\models\chi$. By the inductive assumption, $\M',v\models\tau(\chi)$. Since, by the construction of $R'$, we know that $(w,w_s)\notin R'$, we can derive $\M',w\models\Box\tau(\chi)$. Hence, by the definition of $\tau$, $\M',v\models\tau(\Diamond\chi)$.\smallskip

\noindent $\psi=\E\chi$\quad Assume that $\M,w\models\E\chi$. Then, there exists $v\in W$ such that $\M,v\models\chi$, and moreover, by the definition of $V'$, for which $V'(p_\chi)=\{v\}$. Since $v\in W$, then $v\neq w_s$, and so $\M',v\models\neg s$.
By the inductive assumption we get $\M',v\models\tau(\psi)$. Thus, $v$ is the unique world in $W'$ such that $\M',v\models p_\chi$, and moreover, $\M,v\models\tau(\chi)\land\neg s$ for this $v$. Therefore, $\M',w\models @_{\iota p_\psi} (\tau(\psi)\land\neg s)$, so by the definition of $\tau$ we finally obtain $\M',w\models\tau(\E\chi)$.\smallskip

\noindent $\psi=\A\chi$\quad Assume that $\M,v\models\A\chi$. Then, for all $v\in W$, $\M,v\models\chi$. By the inductive assumption, for all $v\in W$, and so, for all $v\in W'$ such that $v\neq w_s$, we have $\M',v\models\tau(\chi)$. Since $w_s$ is the unique world in $W'$ such that $\M',w_s\models s$, we get that $w_s$ is the unique world such that $\M',w_s\models s\lor\neg\tau(\chi)$. Thus, by the semantics of $@_\iota$, we have $\M',w\models @_{\iota(s\lor\neg\tau(\chi)}\top$, and further, by the definition of $\tau$, we get $\M',w\models\tau(\A\chi)$.\smallskip

Now we will conduct the induction for the opposite direction.\smallskip

\noindent $\psi=p$ or $\psi=\neg p$ \quad Since in this case $\tau(\psi)=\psi$, by the assumption that $\M',w\models\tau(\psi)$, we get $\M,w\models\psi$.\smallskip

\noindent $\psi=\chi\land\theta$\quad Assume that $\M',w\models\tau(\chi\land\theta)$. By the definition of $\tau$ we derive $\M',w\models\tau(\chi)\land\tau(\theta)$, and so $\M',w\models\tau(\chi)$ and $\M',w\models\tau(\theta)$. By the inductive assumption, $\M,w\models\chi$ and $\M,w\models\theta$, and hence, $\M,w\models\chi\land\theta$. The case where $\psi=\chi\lor\theta$ is dealt with similarly.\smallskip

\noindent $\psi = \Diamond\chi$\quad Assume that $\M',w\models\tau(\Diamond\chi)$. By the definition of $\tau$ we get $\M',w\models\Diamond\tau(\chi)$, and so, there exists $v\in W$ such that $(w,v)\in R$ and $\M',v\models\tau(\chi)$. Notice that $w_s\neq v$, as $w_s$ is only accessible from $w_s$ and, by the assumption, $w\neq w_s$. By the inductive assumption we get $\M,v\models\chi$, whence $\M,w \models \Diamond\chi$ follows by the semantics of $\Diamond$. The case where $\psi=\Box\chi$ is handled analogously.\smallskip

\noindent $\psi = \E\chi$\quad Assume that $\M',w\models\tau(\E\chi)$. 
By the definition of $\tau$ it means that $\M',w\models @_{\iota p_\chi} ( \tau(\chi)\land\neg \s )$, where $p_\chi$ is a propositional variable not occurring in $\varphi$. 
By the semantics of $@_\iota$ it means that there exists a unique world $v\in W$ such that $\M',v\models p_\psi$ and, moreover, $\M',v\models\tau(\chi)\land\neg s$ for this $v$. 
By the definition of $V$ we know that $v\neq w_s$, so we can apply the inductive assumption to get $\M,v\models\chi$, whence we obtain $\M,w\models\E\chi$.\smallskip

\noindent $\psi = \A\chi$ Assume that $\M',w\models\tau(\A\chi)$. By the definition of $\tau$ it follows that $\M',w\models @_{\iota (s \lor \neg \tau(\psi)) }\top$. By the semantics of $@_\iota$ it means that there exists a unique world $v$ such that $\M',v\models s\lor\neg\tau(\chi)$ ($\top$ is irrelevant in this case). Since we have $\M',w_s\models s$, and so, $\M',w_s\models s\lor\neg\tau(\chi)$, it follows that $v=w_s$. Thus, we know that, for any world $u\neq w_s$ it holds that $\M,u\not\models s\lor\neg\tau(\chi)$, and further, $\M',u\not\models\neg\tau(\chi)$, which finally results in $\M',u\models\tau(\chi)$. Thus, for any $u\in W'$, $\M',u\models\tau(\chi)$. We may apply the inductive assumption and obtain $\M,u\models\chi$ for any $u\in W'$, and so, $\M,w\models\A\chi$, as required.
\qed
\end{proof}

%\subsection*{Proof of \Cref{bisim}}

\noindent\textbf{\Cref{bisim}}\quad
\emph{If $\M, w  \leftrightarroweq_\iota \M', w'$ then for any $\MLi$-formula $\varphi$ it holds that $\M, w \models \varphi$ if and only if $\M', w' \models \varphi$.}\medskip

\begin{proof}
Assume that $Z$ is a $\iota$-bisimulation between models $\M=(W,R,V)$ and $\M'=(W',R',V')$ which witnesses the fact that $\M, w  \leftrightarroweq_\iota \M', w'$.
We will show the equivalnce from the theorem inductively on the structure of  $\varphi$.

The base case (when $\varphi$ is a propositional variable) and the inductive step for 
$\varphi$ of the forms $\neg \psi$, $\psi_1 \land \psi_2$, and $\Diamond \psi$ can be shown in the same way as in the
Bisimulation Invariance Lemma for basic modal logic \cite{blackburn2002modal,blackburn2006handbook}.

The remaining (and interesting) case in the inductive step is when $\varphi$ is of the form $@_{\iota \psi_1} \psi_2$.
Assume that 
$\M ,w \models @_{\iota \psi_1} \psi_2$, so there exists a unique world $v \in W$ such that $\M, v \models \psi_1$, and moreover $\M, v \models \psi_2$.
As $Z$ is a $\iota$-bisimilation, it is serial, and thus,
there exists $v' \in W'$ such that $v' \in Z(v)$.
Hence,
by the inductive assumption, $\M' , v' \models \psi_1 \land \psi_2$.
Now, suppose towards a contradiction that
$\M' ,w' \not\models @_{\iota \psi_1} \psi_2$, so
there is $u' \in W'$ such that  $u' \neq v'$ and $\M' , u' \models \psi_1$.
Since $Z$ is a $\iota$-bisimulation, it is surjective, and so, there exists $u \in W$ such that $u' \in Z(u)$.
Moreover, by the inductive assumption we obtain that $\M,u \models \psi_1$.
However, $v$ is the only world in $W$ which satisfies $\psi_1$, so $u=v$ and consequently $u' \in Z(v)$.
For the same reason there cannot be in $W$ any  world different than $v$ which is mapped by $Z$ to $v'$.
Hence, $Z^{-1}(v') = \{v \}$ and therefore, by the definition of  $\iota$-bisimulation, we obtain that $Z(v) = \{ v' \}$.
This, however, contradicts the fact that $u' \in Z(v)$ and $u' \neq v'$.
As a result we have shown that $\M, w \models \varphi$ implies that $\M', w' \models \varphi$.
The opposite implication is shown analogously, as the defining properties of a $\iota$-bisimulation are symmetric.
\qed
\end{proof}
